# Supplementary material for: SEMDR: A Semantic-Aware Dual Encoder Model for Legal Judgment Prediction with Legal Clue Tracing
Source: arXiv:2408.09717 source file (2024-08-19)
Supplement: Supplementary file 1 [file AppendixD.tex]

\begin{table*}[!t]
\centering
\caption{Judgement prediction on High-frequency Criminal Charge Scenario (CAIL-small).}
\label{cail-small}
\resizebox{\linewidth}{!}{

\begin{tabular}{l|cccc|cccc|cccc} 
\hline
Dataset                  & \multicolumn{12}{c}{CAIL-small}                                                                                                                                                                              \\ 
\hline
\multirow{2}{*}{Methods}    & \multicolumn{4}{c|}{Law Article}                                  & \multicolumn{4}{c|}{Charges}                                      & \multicolumn{4}{c}{Imprisonment}                                   \\ 
\cline{2-13}
                            & Acc            & MP             & MR             & F1             & Acc            & MP             & MR             & F1             & Acc            & MP             & MR             & F1              \\ 
\hline
TF-IDF+SVM                  & 81.56          & 78.68          & 71.55          & 73.89          & 80.20          & 79.04          & 73.23          & 75.16          & 37.61          & 36.71          & 30.87          & 31.93           \\
LSTM                        & 86.69          & 79.99          & 78.07          & 78.43          & 85.95          & 81.81          & 80.94          & 81.07          & 40.35          & 39.61          & 33.93          & 33.96           \\
DPCNN                       & 86.09          & 80.39          & 79.04          & 78.91          & 84.71          & 82.27          & 79.13          & 79.81          & 39.24          & 40.46          & 30.55          & 31.62           \\
NeurJudge                   & 84.17          & 80.99          & 79.57          & 79.86          & 87.40          & 83.28          & 81.19          & 81.71          & 37.64          & 36.43          & 34.65          & 35.33           \\
TextCNN                     & 85.66          & 82.92          & 74.73          & 77.24          & 84.79          & 84.49          & 77.13          & 79.34          & 38.69          & 39.22          & 31.11          & 32.08           \\
TopJudge                    & 87.04          & 85.41          & 78.35          & 80.59          & 85.84          & 85.67          & 79.07          & 81.16          & 38.59          & 36.80          & 34.13          & 31.49           \\
LADAN                       & 89.24          & 84.95          & 79.52          & 78.79          & 86.89          & 82.90          & 81.57          & 82.84          & 40.19          & 34.69          & 35.66          & 35.62           \\
Few-Shot                    & 86.32          & 85.97          & 85.25          & 78.69          & 85.95          & 84.35          & 81.73          & 81.57          & 37.56          & 34.66          & 35.02          & 36.33           \\
BERT                        & 92.23          & 89.20          & 89.04          & 88.97          & 91.56          & 89.66          & 89.61          & 89.49          & 44.34          & 44.60          & 40.46          & 41.05           \\
BERT-Crime                  & 92.54          & 89.64          & 89.34          & 89.15          & 91.88          & 90.01          & 90.52          & 90.44          & 44.59          & 44.78          & 40.70          & 41.14           \\ 
\hline
\textbf{SEMDR}              & \textbf{95.48} & \textbf{95.25} & \textbf{94.93} & \textbf{94.07} & \textbf{94.74} & \textbf{93.59} & \textbf{93.72} & \textbf{94.86} & \textbf{46.35} & \textbf{44.94} & \textbf{45.60} & \textbf{43.98}  \\
\hline
\end{tabular}

}
\end{table*}

\begin{table*}[!t]
\centering
\caption{Judgement prediction on High-frequency Criminal Charge Scenario (CAIL-big). SEMDR has tested three subtasks in the CAIL-small and CAIL-big datasets, which contain 121,045 and 152,744 criminal cases respectively.}
\label{cail-big}
\resizebox{\linewidth}{!}{
\begin{tabular}{l|cccc|cccc|cccc} 
\hline
Dataset                  & \multicolumn{12}{c}{CAIL-big}                                                                                                                                                                              \\ 
\hline
\multirow{2}{*}{Methods} & \multicolumn{4}{c|}{Law Article}                                  & \multicolumn{4}{c|}{Charges}                                      & \multicolumn{4}{c}{Imprisonment}                                   \\ 
\cline{2-13}
                         & Acc            & MP             & MR             & F1             & Acc            & MP             & MR             & F1             & Acc            & MP             & MR             & F1              \\ 
\hline
TF-IDF+SVM                                    & 93.17          & 84.56          & 72.54          & 77.10          & 92.74          & 82.64          & 70.71          & 75.14          & 49.24          & 50.13          & 41.09          & 50.14           \\
LSTM                                          & 95.41          & 84.70          & 85.25          & 84.61          & 95.37          & 85.41          & 84.51          & 84.43          & 54.46          & 41.29          & 38.42          & 38.32           \\
DPCNN                                         & 95.35          & 86.57          & 83.65          & 84.72          & 95.21          & 85.46          & 84.45          & 84.47          & 54.07          & 41.17          & 34.91          & 35.36           \\
NeurJudge                                     & 94.44          & 89.28          & 86.22          & 87.04          & 95.61          & 92.12          & 88.33          & 89.66          & 53.82          & 40.35          & 37.82          & 38.17           \\
TextCNN                                       & 95.21          & 88.91          & 81.20          & 84.29          & 95.06          & 87.95          & 80.90          & 83.55          & 53.47          & 42.49          & 30.94          & 33.02           \\
TopJudge                                      & 94.28          & 85.41          & 75.98          & 80.59          & 93.60          & 85.67          & 74.60          & 81.16          & 52.77          & 36.80          & 34.53          & 34.68           \\
LADAN                                         & 95.48          & 90.01          & 83.53          & 90.08          & 94.44          & 87.81          & 79.95          & 88.86          & 53.26          & 50.97          & 36.73          & 51.77           \\
Few-Shot                                      & 89.63          & 89.45          & 89.05          & 89.41          & 90.22          & 90.35          & 89.87          & 90.04          & 50.01          & 48.76          & 49.63          & 49.42           \\
BERT                                          & 96.35          & 95.82          & 96.21          & 95.44          & 97.06          & 96.37          & 96.88          & 96.47          & 55.88          & 54.96          & 55.71          & 54.67           \\
BERT-Crime                                    & 96.37          & 96.07          & 94.67          & 95.58          & 96.69          & 96.65          & 95.03          & 96.49          & 55.59          & \textbf{55.20} & 54.81          & 54.94           \\ 
\hline
\textbf{SEMDR}                                & \textbf{96.53} & \textbf{96.11} & \textbf{96.26} & \textbf{96.31} & \textbf{97.78} & \textbf{96.81} & \textbf{97.27} & \textbf{96.64} & \textbf{55.97} & 55.16          & \textbf{56.25} & \textbf{55.42}  \\
\hline
\end{tabular}
}
\end{table*}
