# Supplementary material for: SEMDR: A Semantic-Aware Dual Encoder Model for Legal Judgment Prediction with Legal Clue Tracing
Source: arXiv:2408.09717 source file (2024-08-19)
Supplement: Supplementary file 2 [file AppendixA.tex]

\begin{figure}[!t]
\centering 
\subfigure[The Standard Format of Legal Judgment Documents.\label{app_a1}]{
    \includegraphics[scale=0.16]{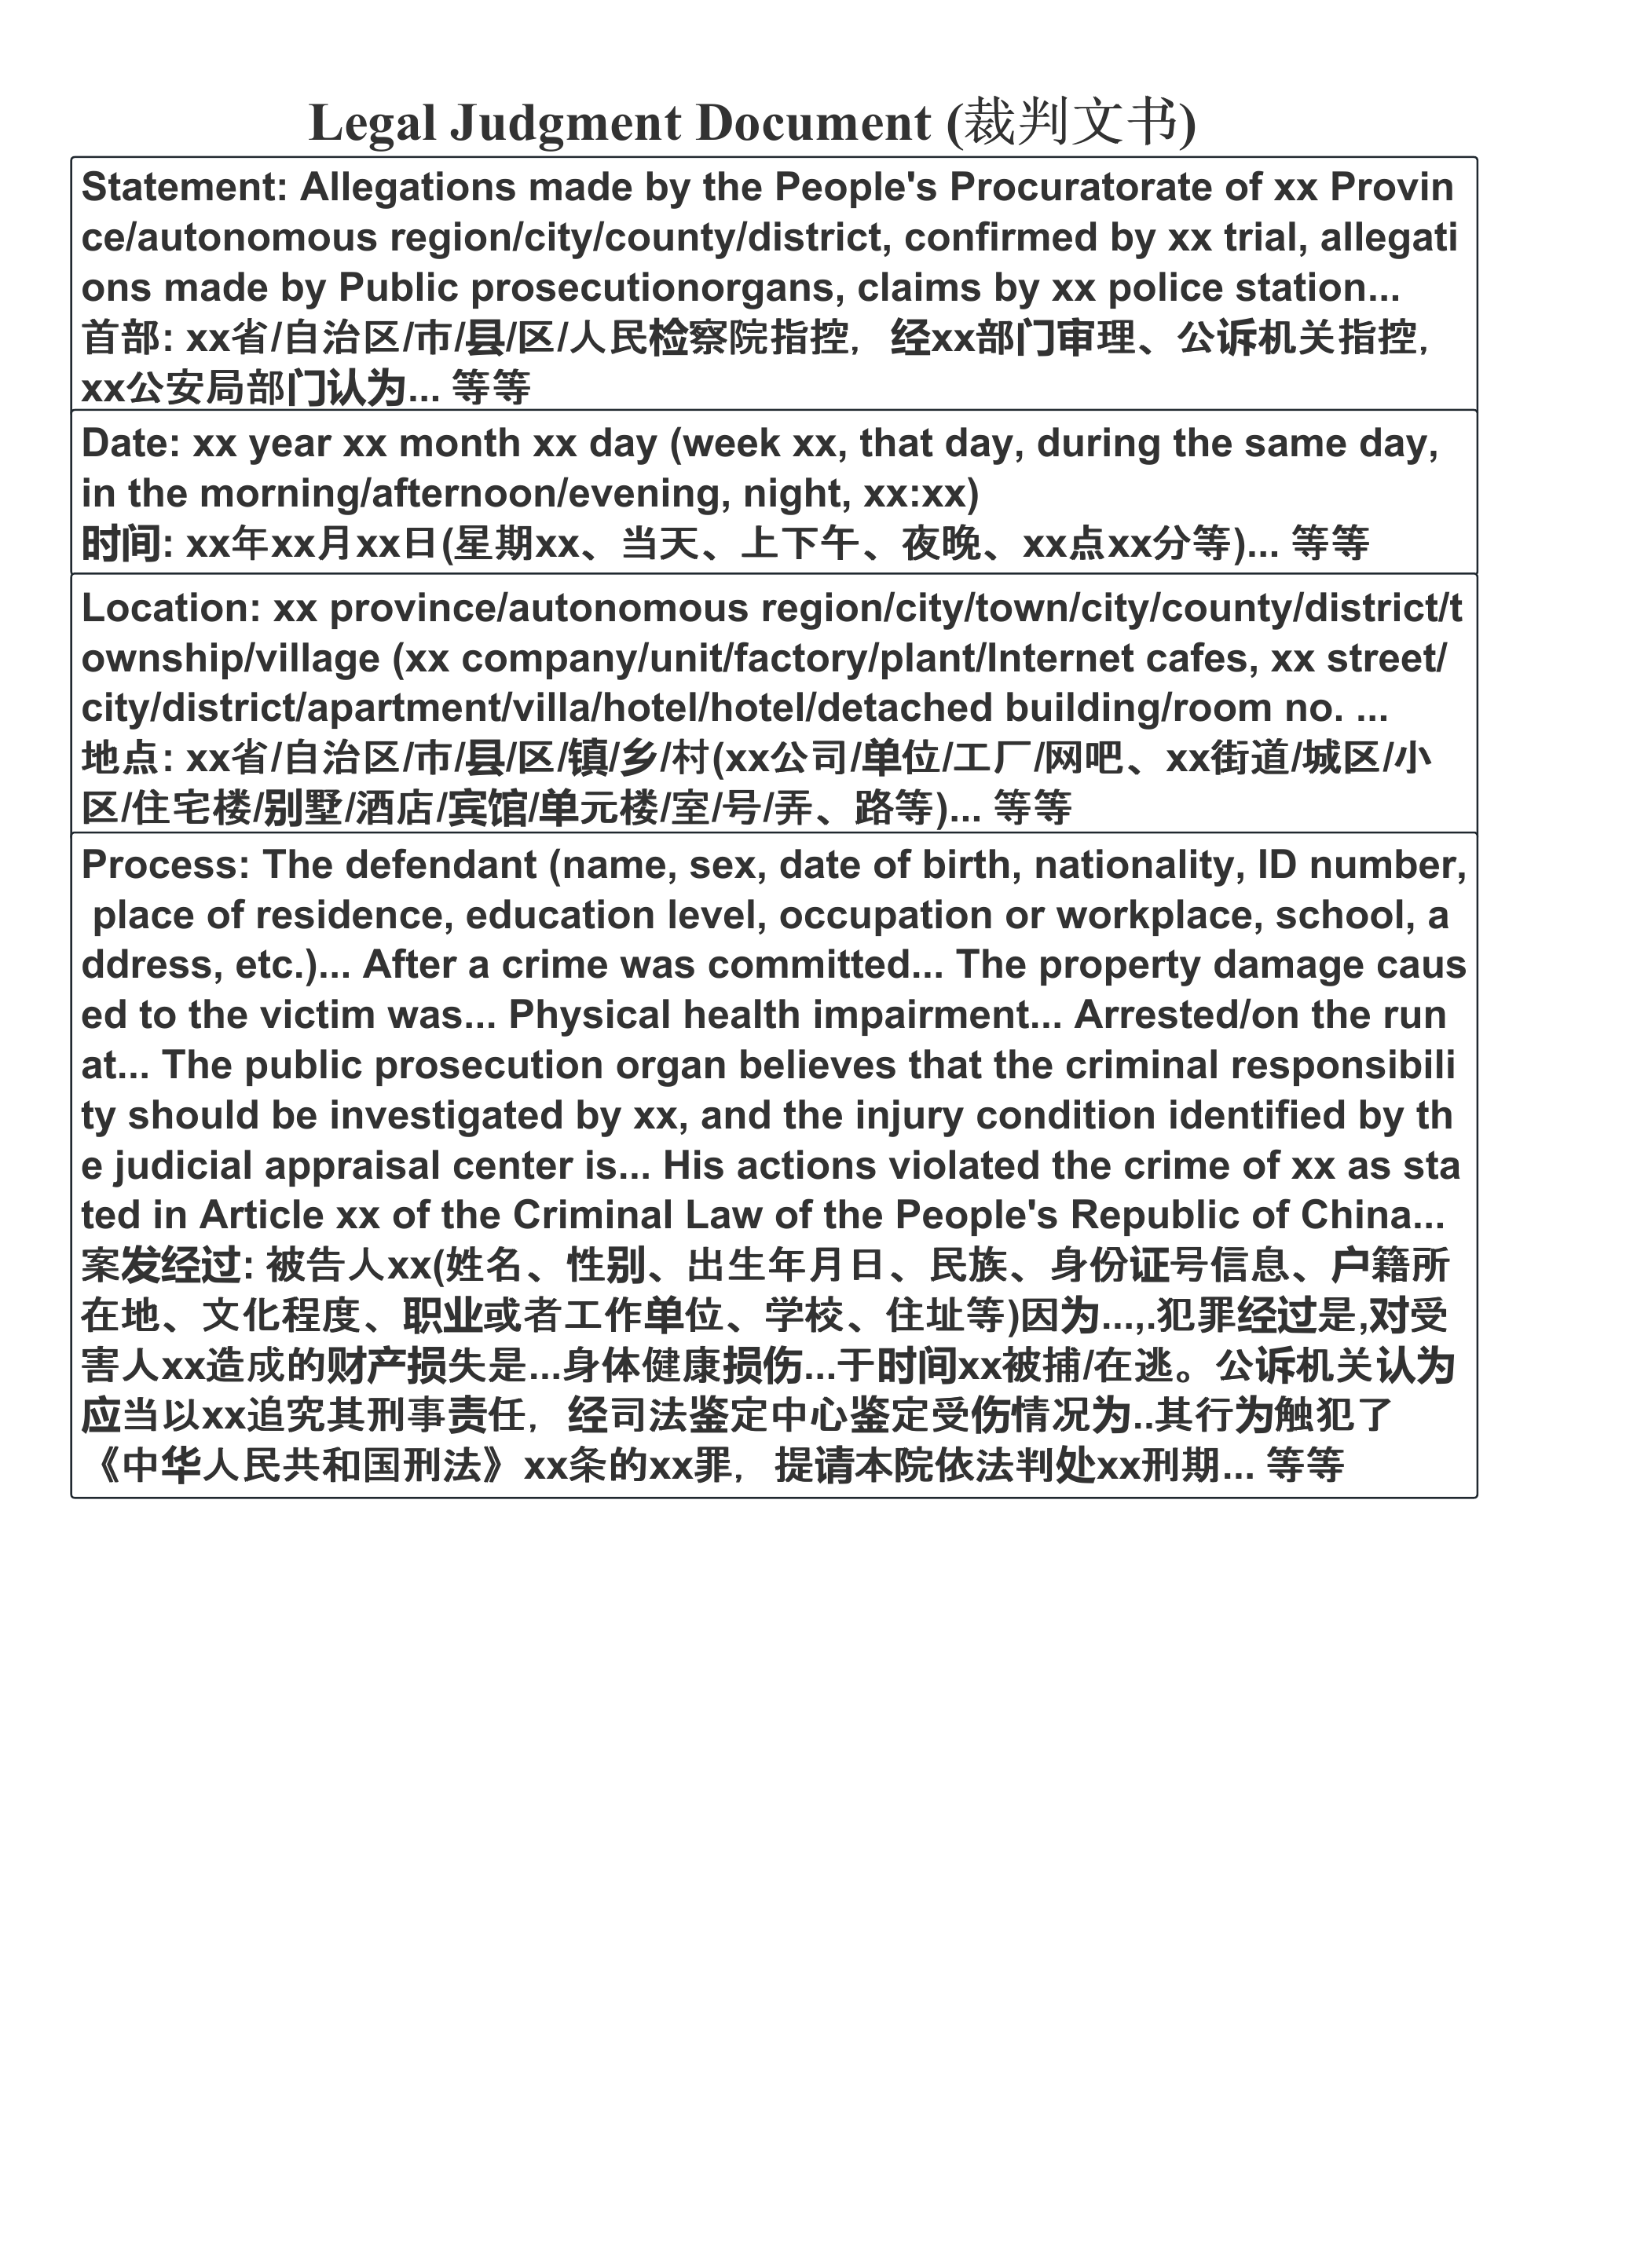}
}
\hfill 
\subfigure[An Example of Lexicon-Tracing Method.\label{app_a2}]{
    \includegraphics[scale=0.18]{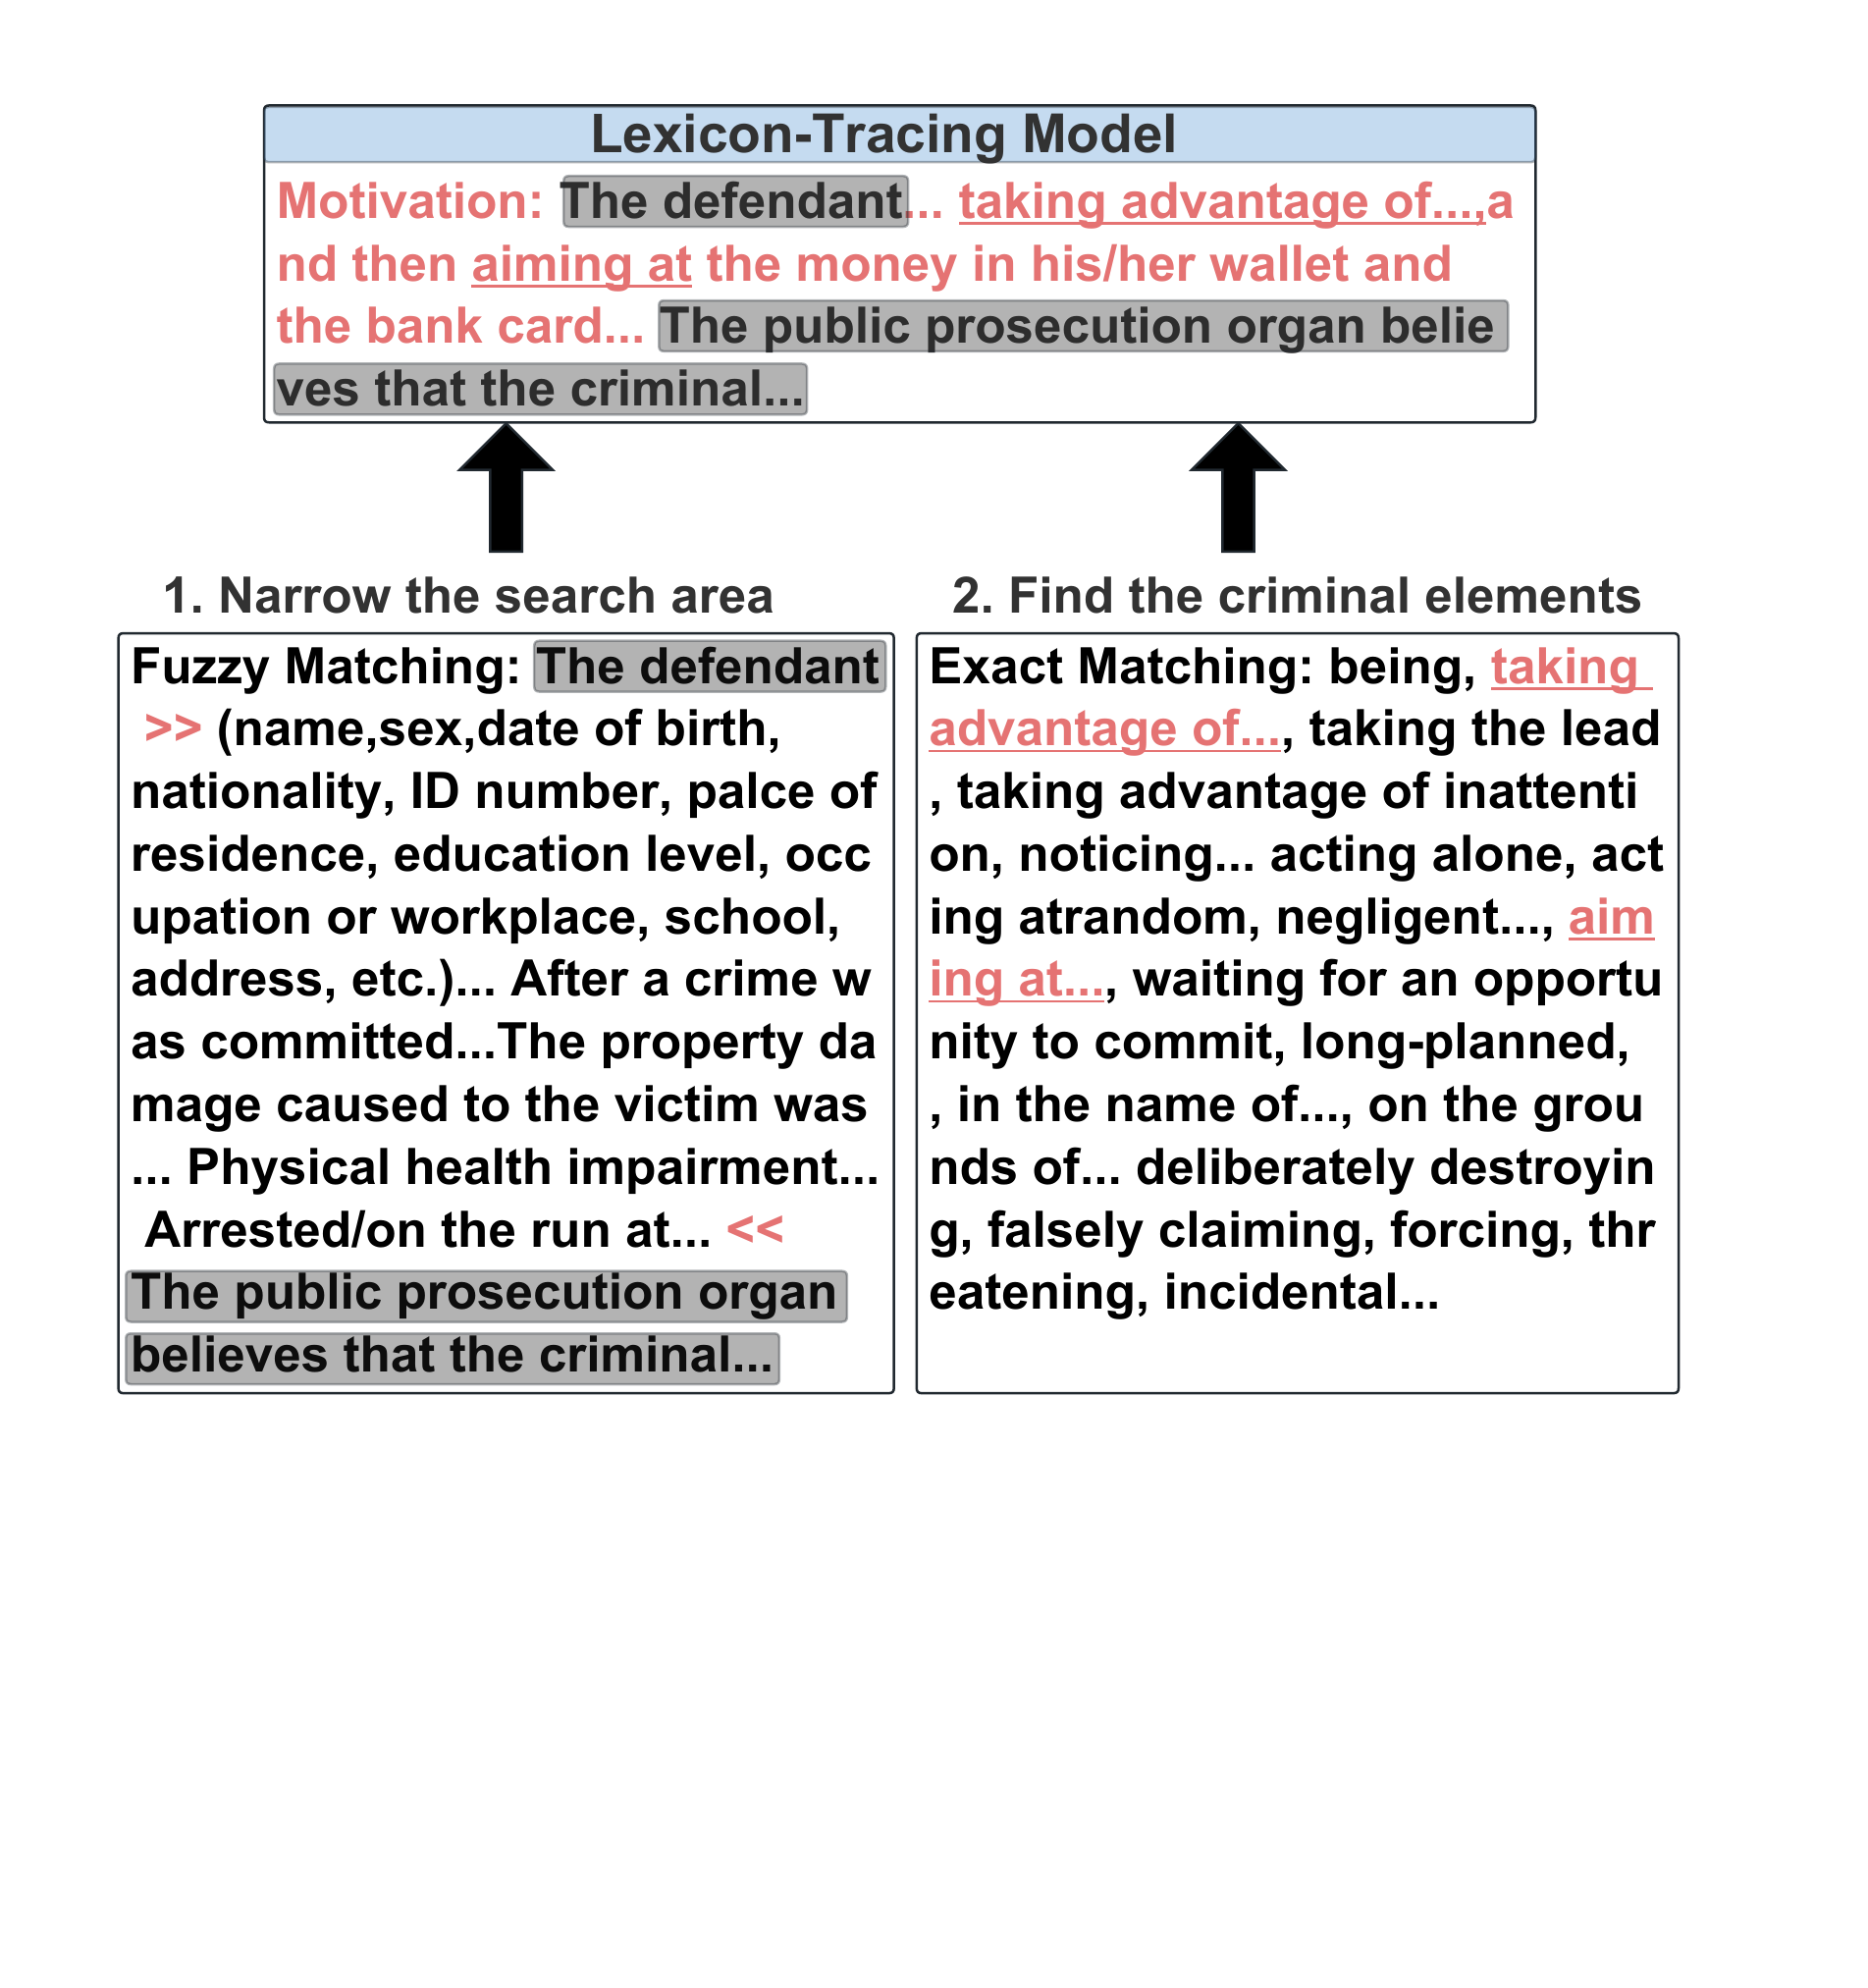}
}
\caption{SEMDR's Fine-Grained Analysis at the Lexicon Level.}
\vspace{-8mm}  % Adjust vertical space as needed
\end{figure}
