# Supplementary material for: SEMDR: A Semantic-Aware Dual Encoder Model for Legal Judgment Prediction with Legal Clue Tracing
Source: arXiv:2408.09717 source file (2024-08-19)
Supplement: Supplementary file 3 [file AppendixB.tex]

\begin{figure}[t]
    \includegraphics[width = 1\linewidth] {./Figures/appenix23.pdf}
    \caption{\label{app_b1}The Nodes and Relations in the Legal Judgment Reasoning Graph.}
\end{figure}
